# Supplementary material for: Learning Neural Networks with Two Nonlinear Layers in Polynomial Time
Source: arXiv:1709.06010 source file (2018-04-20)
Supplement: Supplementary file 1 [file appendix.tex]

\section{Alphatron-u} \label{sec:alphatron-u}
For the case of unknown $u$, we propose the algorithm Alphatron-u similar to the SLIsotron algorithm by \cite{KKKS11}.

\begin{algorithm}[H]
\caption{Alphatron-u}\label{Alphatron-u}
    \SetKwInOut{Input}{Input}
    \SetKwInOut{Output}{Output}
    \Input{data $\langle (\textbf{x}_\textbf{i}, y_i \rangle_{i=1}^m \in \mathbb{R}^n \times [0,1]$, $u: \mathbb{R} \rightarrow [0,1]$, kernel function $K$ corresponding to feature map $\psi$, learning rate $\lambda > 0$, held-out data $\langle (\textbf{a}_\textbf{j}, b_j \rangle_{j=1}^s \in \mathbb{R}^n \times [0,1]$}
    $\alpha^1 := 0 \in \mathbb{R}^m$\\
    \For{$t = 1, 2, \ldots$}{
    $f^t(x) := \sum_{i=1}^m \alpha_i^t K(x, \textbf{x}_\textbf{i})$\\
    $u^t := \text{LIR}((f^t(\textbf{x}_\textbf{i}), y_i), \ldots, (f^t(x_m), y_m))$\\
    $h^t(x) := u^t(f^t(x))$\\
    \For{$i = 1,2, \ldots, m$}{
    $\alpha^{t+1}_i := \alpha^t_i + \frac{\lambda}{m}(y_i - h^t(\textbf{x}_\textbf{i}))$
    }
    }
    \Output{$\argmin_{h^t} \sum_{j=1}^s(h^t(\textbf{a}_\textbf{j}) - b_j)^2$}
\end{algorithm}

Note that LIR is Lipschitz Isotonic Regression which fits a 1D Lipschitz monotonic function in the direction of $v^t$ over the predicted labels $f^t(\cdot)$ by minimizing the distance to the actual labels $y$. We refer the reader to \cite{KKKS11} for a detailed description of the algorithm and the procedure. We use the following lemma for LIR from their paper for our analysis.
\begin{lemma}[\cite{KKKS11}] \label{lem:lir}
Let $(z_i, y_i)_{i=1}^m$ be input to LIR where $z_i$ are decreasing and $y_i \in [0,1]$. Let $\hat{y}_1, \ldots, \hat{y}_m$ be the output of LIR. For any function $f$ such that $f(b) - f(a) \geq b - a$ for $b \geq a$ then,
\[
\sum_{i=1}^m (y_i - \hat{y}_i)(f(\hat{y}_i) - z_i) \geq 0.
\]
\end{lemma}
\subsection{Analysis}
\begin{theorem} \label{thm:Alphatron-u}
Let $K$ be a kernel function corresponding to feature map $\psi$ such that for all $\textbf{x}$, $||\psi(\textbf{x})|| \leq 1$. Consider samples $(\textbf{x}_\textbf{i},y_i)_{i=1}^m$ drawn iid from $\mathbb{R}^n \times [0,1]$ such that $E[y|\textbf{x}] = u(\langle \textbf{v}, \psi(\textbf{x}) \rangle + \xi(x))$ where $u: \mathbb{R} \rightarrow [0,1]$ is an unknown $L$-Lipschitz non-decreasing function, $\xi: \mathbb{R}^n \rightarrow [-\epsilon_0, \epsilon_0]$ for $\epsilon_0\in(0,1)$ and $||\textbf{v}|| \leq B$. Then for $\delta \in (0,1)$, with probability $1 - \delta$, for some $t < O(BL/\eta)$,
\[
\varepsilon(h^t) \leq O(L\epsilon_0 + BL\eta)
\]
where $\eta$ equals 
% dimension dependent $\left(\frac{n(BL)^2\log(BLm/\delta)}{m}\right)^{1/3}$ or dimension independent 
$\left(\frac{(BL)^2\log(m/\delta)}{m}\right)^{1/4}$
\end{theorem}
We follow the analysis of \cite{KKKS11} while giving the modifications. We redefine $\textbf{v}^\textbf{t} = \sum_{i=1}^m \alpha_i^t \psi(\textbf{x}_\textbf{i})$ giving us that $f^t(x) = \langle \textbf{v}^t, \psi(x) \rangle$. We further define 
\[
\forall i \ \hat{y}_i^t = h^t(\textbf{x}_\textbf{i}) = u^t(f^t(\textbf{x}_\textbf{i})).
\]
Define,
\[
\forall i \ \bar{y}_i =  u(\langle \textbf{v}, \psi(\textbf{x}_\textbf{i}) \rangle  + \xi(\textbf{x}_\textbf{i}).
\]
% and
% \[
% \forall i \ \check{y}_i =  u(\langle \textbf{v}, \psi(\textbf{x}_\textbf{i}) \rangle)).
% \]
% Observe that $\forall i |\check{y}_i - \bar{y}_i| \leq L \epsilon_0$. 
Consider a call to LIR on inputs $(f^t(\textbf{x}_\textbf{i}), \check{y}_i)_{i=1}^m$ giving output $\tilde{u}^t$. Define
\[
\forall i \ \tilde{y}_i^t =  \tilde{u}^t(f^t(\textbf{x}_\textbf{i})).
\]
Using the above notation, we give the following lemma central to our analysis.
\begin{lemma} \label{lem:Alphatron-u}
At iteration $t$ in Alphatron-u, suppose $||\textbf{v}^\textbf{t} - \textbf{v}|| \leq B$ for $B > 1$ and $||(1/m) \sum_{i=1}^m(y_i - \bar{y}_i)\psi(\textbf{x}_\textbf{i})|| \leq \eta_1$ and $(1/m) \sum_{i=1}^m|\hat{y}_i^t - \tilde{y}_i^t| \leq \eta_2$, then
\[
 ||\textbf{v}^\textbf{t} - \textbf{v}||^2 - ||\textbf{v}^\textbf{t+1} - \textbf{v}||^2 \geq \lambda \left(\left( \frac{1}{L} - \lambda \right)\hat{\varepsilon}(h^t)  -2B\eta_1 - 2B\eta_2- 2 \epsilon_0  -\lambda\eta_1^2 -\frac{2}{L} \eta_2 - 2\lambda \eta_1\right)
\]
\end{lemma}
\begin{proof}
We have,
\begin{align}
||\textbf{v}^\textbf{t} - \textbf{v}||^2 &- ||\textbf{v}^\textbf{t+1} - \textbf{v}||^2 \nonumber\\
& \geq \frac{2\lambda}{m}\sum_{i=1}^m(y_i - \hat{y}_i^t)\langle \textbf{v} - \textbf{v}^\textbf{t}, \psi(\textbf{x}_\textbf{i})\rangle - \lambda^2\left|\left| \frac{1}{m} \sum_{i=1}^m (y_i - \hat{y}_i^t)\psi(\textbf{x}_\textbf{i})\right|\right|^2  \label{eq:expand}\\
& \geq \frac{2\lambda}{m}\sum_{i=1}^m(y_i - \bar{y}_i)\langle \textbf{v} - \textbf{v}^\textbf{t}, \psi(\textbf{x}_\textbf{i})\rangle + \frac{2\lambda}{m}\sum_{i=1}^m(\bar{y}_i - \tilde{y}_i^t)\langle \textbf{v} - \textbf{v}^\textbf{t}, \psi(\textbf{x}_\textbf{i})\rangle \nonumber\\
&\ + \frac{2\lambda}{m}\sum_{i=1}^m(\tilde{y}_i^t - \hat{y}_i^t)\langle \textbf{v} - \textbf{v}^\textbf{t}, \psi(\textbf{x}_\textbf{i})\rangle - \lambda^2\left|\left| \frac{1}{m} \sum_{i=1}^m (y_i - \hat{y}_i^t)\psi(\textbf{x}_\textbf{i})\right|\right|^2 \label{eq:sep}\\
& \geq -2\lambda B\eta_1 + \frac{2\lambda}{m}\sum_{i=1}^m(\bar{y}_i - \tilde{y}_i^t)\langle \textbf{v} - \textbf{v}^\textbf{t}, \psi(\textbf{x}_\textbf{i})\rangle - 2\lambda B\eta_2 - \lambda^2\left|\left| \frac{1}{m} \sum_{i=1}^m (y_i - \hat{y}_i^t)\psi(\textbf{x}_\textbf{i})\right|\right|^2 \label{eq:bound}
\end{align}
(\ref{eq:expand}) follows from $\textbf{v}^\textbf{t+1}-\textbf{v}^\textbf{t} = (1/m)\sum_{i=1}^m(y_i - \hat{y}_i^t)\psi(\textbf{x}_\textbf{i})$, (\ref{eq:bound}) follows from bounding the first and third term using the assumptions. We will bound the second and fourth term as follows. Assuming for simplicity that $u$ is strictly increasing (inverse exists),

\begin{align}
\frac{2}{m}\sum_{i=1}^m(\bar{y}_i - \tilde{y}_i^t)\langle \textbf{v} - \textbf{v}^\textbf{t}, \psi(\textbf{x}_\textbf{i})\rangle &= \frac{2}{m}\sum_{i=1}^m(\bar{y}_i - \tilde{y}_i^t)(\langle \textbf{v}, \psi(\textbf{x}_\textbf{i})\rangle + \xi(\textbf{x}_\textbf{i}) - u^{-1}(\tilde{y}_i^t))\nonumber\\
&\  - \frac{2}{m}\sum_{i=1}^m(\bar{y}_i - \tilde{y}_i^t)\xi(\textbf{x}_\textbf{i}) + \frac{2}{m}\sum_{i=1}^m(\bar{y}_i - \tilde{y}_i^t)(u^{-1}(\tilde{y}_i^t) - \langle \textbf{v}^t, \psi(\textbf{x}_\textbf{i})\rangle) \\
&\geq \frac{2}{m}\sum_{i=1}^m(\bar{y}_i - \tilde{y}_i^t)(u^{-1}(\bar{y}_i) - u^{-1}(\tilde{y}_i^t))  - 2\epsilon_0 \label{eq:gamma}\\
&\geq \frac{2}{Lm} \sum_{i=1}^m (\bar{y}_i - \tilde{y}_i^t)^2 - 2 \epsilon_0 \label{eq:eh}\\
&\geq \frac{2}{Lm} \sum_{i=1}^m (\bar{y}_i - \hat{y}_i^t + \hat{y}_i^t - \tilde{y}_i^t)^2 - 2 \epsilon_0\\
&\geq \frac{1}{Lm} \sum_{i=1}^m (\bar{y}_i - \hat{y}_i^t)^2 - \frac{2}{Lm}(\hat{y}_i^t - \tilde{y}_i^t)^2 - 2 \epsilon_0 \label{eq:tri}\\
& \geq \frac{1}{L}\hat{\varepsilon}(h^t) - \frac{2\eta_2}{L} - 2 \epsilon_0 \label{eq:tilde}
\end{align}
Here (\ref{eq:gamma}) follows from bounding norm of $\xi$ and observing that $\frac{2}{m}\sum_{i=1}^m(\bar{y}_i - \tilde{y}_i^t)(u^{-1}(\tilde{y}_i^t) - \langle \textbf{v}^t, \psi(\textbf{x}_\textbf{i})\rangle)$ is positive by applying Lemma \ref{lem:lir} for $f = u^{-1}$. (\ref{eq:eh}) follows from the lipschitzness of $u$. (\ref{eq:tri}) follows from $(a + b)^2 \geq a^2/2 - b^2$ for all $a,b \in \mathbb{R}$ and (\ref{eq:tilde}) follows from the bound given by $\eta_2$. Note that this argument generalizes to non-decreasing $u$.

We complete the proof by bounding the fourth term similar to the proof of Lemma \ref{lem:alphatron} as
\begin{align}
\left|\left| \frac{1}{m} \sum_{i=1}^m (y_i - \hat{y}_i^t)\psi(\textbf{x}_\textbf{i})\right|\right|^2 \leq  \hat{\varepsilon}(h^t) + \eta_1^2 +2\eta_1.
\end{align}
\end{proof}

Since $(y_i - \bar{y}_i)\psi(\textbf{x}_\textbf{i})$ are 0-mean iid random variables bounded in norm by 1, we have by the Hoeffding's inequality that 
\[
\left|\left|\frac{1}{m} \sum_{i=1}^m(y_i - \bar{y}_i)\psi(\textbf{x}_\textbf{i})\right|\right| \leq \frac{1}{\sqrt{m}} \left( 1 + \sqrt{2 \log(1/\delta)}\right).
\]
Thus we can set $\eta_1 = \frac{1}{\sqrt{m}} \left( 1 + \sqrt{2 \log(1/\delta)}\right)$. We bound $\eta_2$ using the following theorem from \cite{KKKS11} with a slight modification.

\begin{theorem}
Let $\mathcal{U} = \{u:[-W,W] \rightarrow [0,1]: u\ L\text{-Lipschitz}\}$
\end{theorem}

\[
\eta_2 = 
% \min \left\lbrace O\left(\left(\frac{n(BL)^2\log(BLm/\delta)}{m}\right)^{1/3}\right),
O\left(\left(\frac{(BL)^2\log(m/\delta)}{m}\right)^{1/4}\right).
% \right\rbrace.
\]
Now setting $\lambda = 2/L$ and using a similar argument as of the proof of Lemma \ref{lem:alphatron}, we get that in at most $BL/(\eta_1 + \eta_2)$ iterations we get for some $T$, $\hat{\varepsilon}(h^T) \leq O(L\epsilon_0 + BL(\eta_1 + \eta_2))$ giving us the desired result.

Similar to Alphatron, we can find such a hypothesis by sampling $s = \log(T/\delta)/\epsilon^2$ fresh samples and computing the minimum.
